# Supplementary material for: Methods for Mitigating Uncertainty in Real-Time Operations of a Connected Microgrid
Source: arXiv:2409.19568 source file (2024-09-29)
Supplement: Supplementary file 1 [file appendix.tex]

% \appendix
% \section{My Appendix}
% Appendix sections are coded under \verb+\appendix+.

% \verb+\printcredits+ command is used after appendix sections to list 
% author credit taxonomy contribution roles tagged using \verb+\credit+ 
% in frontmatter.

% \printcredits
